# Supplementary material for: Phonon thermal transport shaped by strong spin-phonon scattering in a Kitaev material Na$_2$Co$_2$TeO$_6$
Source: arXiv:2306.16963 source file (2023-06-29)
Supplement: Supplementary file 1 [file NCTO_LT_SM.pdf]

### Supplementary Materials for:

# Phonon thermal transport shaped by strong spin-phonon scattering in a Kitaev material $Na_2Co_2TeO_6$

## Supplementary Note 1: Additional $\kappa/T(T)$ data.

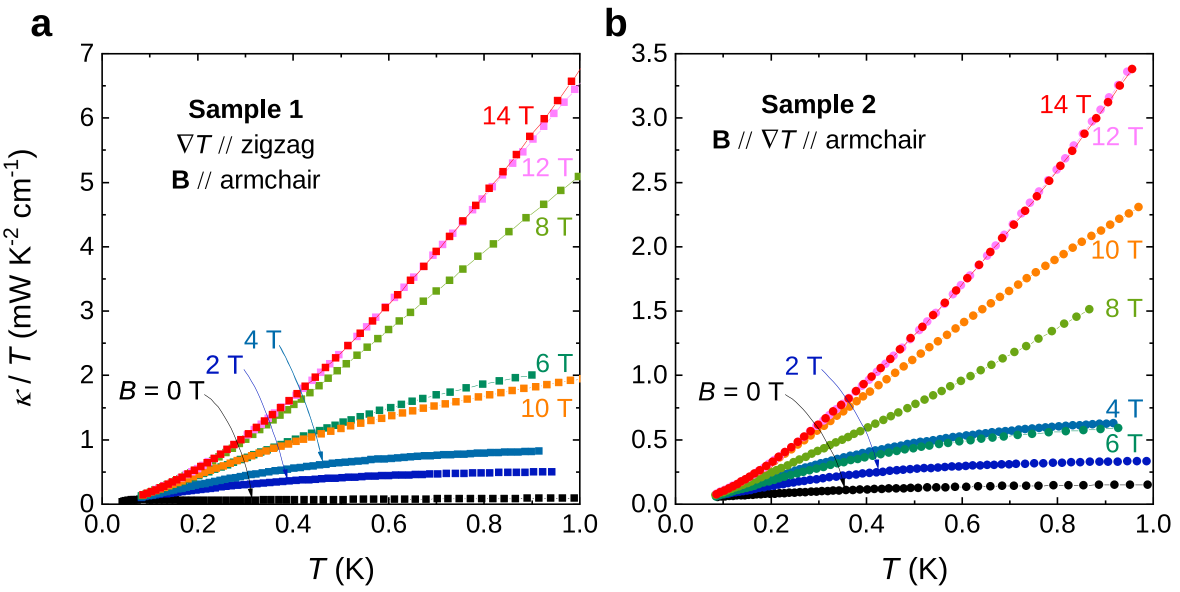


**Supplementary Figure 1 | The $\kappa/T(T)$ curves of two samples with field applied along the *armchair* direction. a,** Sample#1. **b,** Sample#2.

Supplementary Fig. 1 shows the field dependent $\kappa/T(T)$ curves of two crystals, for $\mathbf{B} \parallel$ *armchair* direction. They have similar behavior as the results shown in Fig. 1c of the main text, in that field increases $\kappa$ non-monotonically, until it reaches the saturation field. The data of Sample#1 (Supp. Fig. 1a) was collected on the same sample measured for Fig. 1c with intact thermal contacts. Only the magnetic field direction is rotated from the *zigzag* direction to the *armchair* direction.

## Supplementary Note 2: Additional $\kappa/T(B)$ data and discussion on the hysteresis behavior.

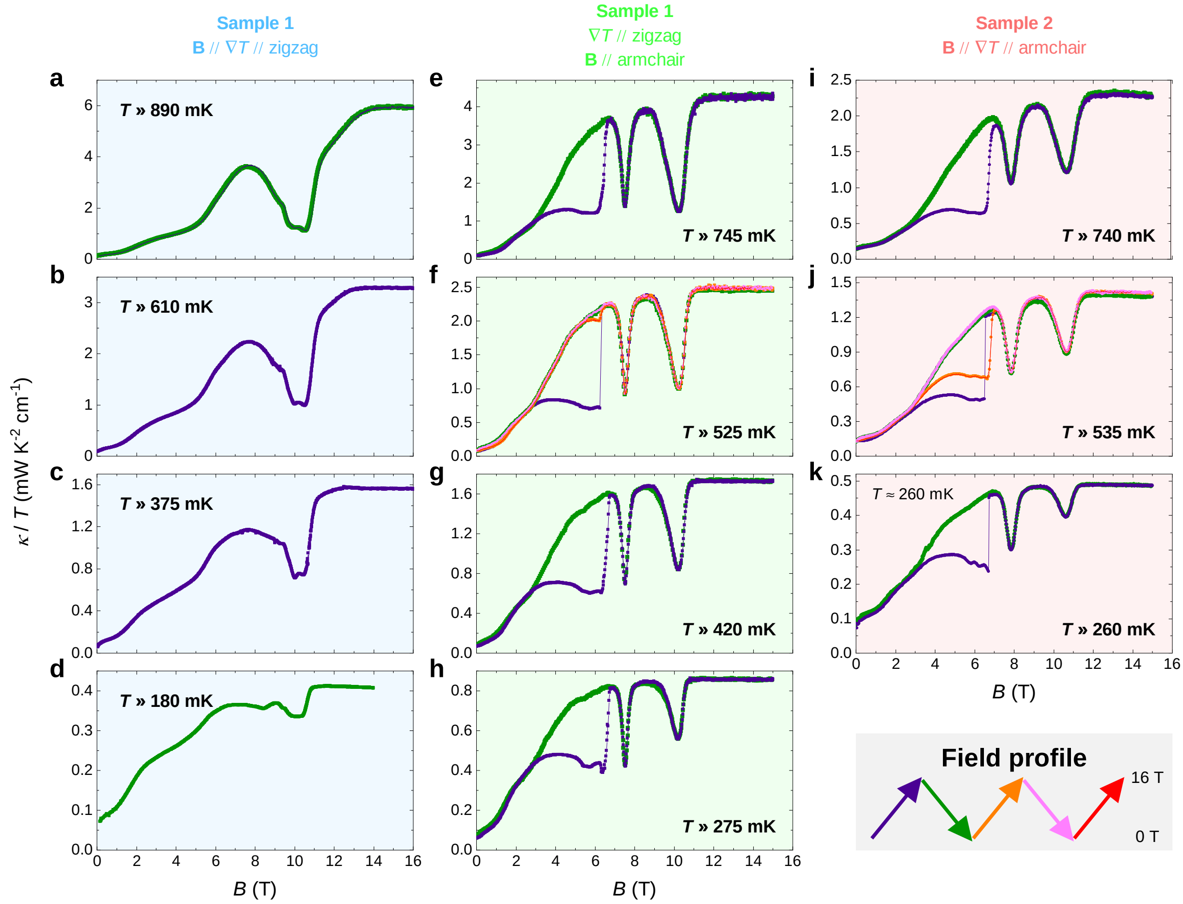


**Supplementary Figure 2 | The $\kappa/T(B)$ isotherms with different combinations of $(\nabla T, B)$ orientations.** Different background colour stands for different $(\nabla T, B)$ orientations as specified on the top of the panels. The data in the blue column (**a - d**) and the green column (**e - h**) were collected on the same crystal after reorienting the field direction. The gray box at the right-bottom corner depicts how the field was applied, at each fixed temperature, after zero field cooling from the paramagnetic higher temperature phase. The data are plotted in violet for the first up-field ramp. Before warming up above 1 K, the second ramp from high field to zero field was plotted in olive, followed by the orange (ramp up), magenta (ramp down), and the red (ramp up) curves.

As shown in Supplementary Fig. 2a, we cannot resolve any hysteresis for **B** applied along

the *zigzag* direction.

When $\mathbf{B}$ is applied along the *armchair* direction, the hysteresis behavior is evident between 3 T to 6.5 T. Magnetic field was ramped up and down at selected temperatures (Supp. Fig. 2f and 2j) for both samples. In both cases, one can see the second up-ramp $\kappa/T(B)$ curve after the saturation field has been reached is different from the first up-ramp $\kappa/T(B)$ curve, but overlaps with the third up-ramp $\kappa/T(B)$ curve. The down-ramp $\kappa/T(B)$ curves are never affected. Obviously, a field hysteresis and the sudden jump of $\kappa$ for the up-field ramp at around 6.5 T point to a first-order transition with a large energy barrier between the two valleys of the energy landscape. We propose two possible mechanisms that can lead to such observation:

**Scenario A**: The magnetically ordered phases of NCTO are different in the low ($\mathbf{B}_{||armchair} < 3$ T) field region and the higher ($\mathbf{B}_{||armchair} > 6.5$ T) field region, and mix in the intermediate field range of 3 T $< \mathbf{B}_{||armchair} <$ 6.5 T. The corresponding states have different excitation DOS at (small) finite temperatures, which induce different phonon scattering strengths. These two states are separated by a large energy barrier. In the field range of 3 T $< \mathbf{B}_{||armchair} <$ 6.5 T, both states are locally stable. During the first up-field ramp, the system is distributed into the two states according to their energy landscape. Applying field $\mathbf{B} \parallel$ *armchair* helps to populate the state with lower DOS. The dominance of the lower DOS state prevails until the system enters the $\mathbf{B}_{||armchair} < 3$ T state again in the down-field ramp. However, as Supp. Fig. 2f and Supp. Fig. 2j indicate, the system remembers whether a field polarized state has been reached. For Sample#1 (Supp. Fig. 2f), the second (orange) and third (red) up-field ramp curves overlap, and the hysteresis region is much reduced to 5.5 T $< \mathbf{B}_{||armchair} <$ 6.5 T. For Sample#2 (Supp. Fig. 2j), the second and third up-field ramp curves also overlap. The hysteresis region is altered compared to the first up-field ramp but is still very large. This sample dependent feature should not be intrinsic but related to details like defects and imperfections in each crystal.

**Scenario B**: NCTO in the field range of 3 T $< \mathbf{B}_{||armchair} <$ 6.5 T is characterized by a unique magnetic order, with different domains, *e.g.*, of a canted *zigzag* phase. The system is expected to develop an approximately equal distribution of domains for small fields. The domain boundaries can scatter phonons, if the domain size is not less than the phonon wavelength, estimated to be of the order of 1 $\mu$m at the relevant temperature range. When

the system re-enter this 3 T $< \mathbf{B}_{\|armchair} <$ 6.5 T phase from high field ($\mathbf{B} \parallel armchair$), one of the domains is preferred. As a result, the overall domain boundary is reduced, thus increases $\kappa$. Pinning effect helps the system to preserve the unequally populated domains to some extent (in a sample dependent manner) when entering this 3 T $< \mathbf{B}_{\|armchair} <$ 6.5 T phase again from the zero-field state.

**To distinguish between the two scenarios** is beyond the scope of the current paper. For this purpose, a careful field dependent heat capacity ($C_p$) measurement at very low temperature is desired. Since domain boundaries are thermodynamically trivial, $C_p$ is expected to be hysteretic in the range of 3 T $< \mathbf{B}_{\|armchair} <$ 6.5 T for **Scenario A**, while is not expected by **Scenario B**.

## Supplementary Note 3: Possible huge heat capacitance in the zero-field phase of NCTO in the low temperature limit.

Our raw data already show some indirect evidences for huge heat capacitance in the zero-field phase of NCTO. As Supplementary Fig. 3 shows, the system needs a very long time to reach thermal equilibrium at zero field, after the system status is changed. When the system is driven to the polarized phase (16 T, for example), the time needed for thermal equilibrium is greatly reduced. Note that in the relevant temperature range (sample temperature less than 100 mK), the thermal conductivity is nearly field independent (See Fig. 1b), so the time needed for achieving a stead-state heat flow can be roughly estimated as a gauge for the heat capacity. Obviously, the larger sample heat capacity, the longer the system needs to reach thermal equilibrium. Taken together, our raw data indeed suggest that the ground state of NCTO at zero field has huge heat capacity, which is greatly reduced in the field polarized state. This indicates a very large DOS of localized magnetic excitations in the zero-field phase.

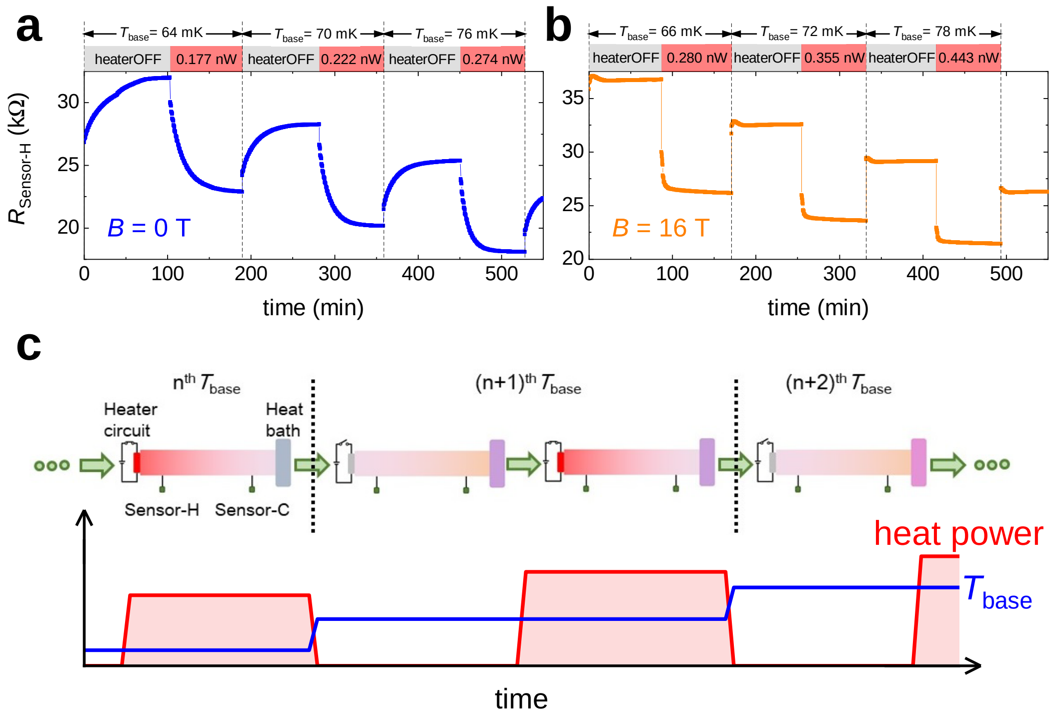


**Supplementary Figure 3 | Raw data of a representative thermometer during a typical measurement in different fields.** The time profile of the resistance of a thermometer (RX-102 $RuO_2$ bare chip from Lakeshore Inc.) **a,** at zero field and **b,** at 16 T (in-plane). The measurement was performed in the "self-calibrated" manner, that is to collect the resistance values of the thermometer with sample heater OFF (for calibration) and with sample heater ON (for calculating $\kappa$) during the same heating-up process. The base temperature ($T_{base}$) was kept constant for each step, and the system is left to reach thermal equilibrium until the data were collected. The presented results are collected during the thermal equilibrium process. The sample heater status is indicated by the alternative gray and pink bars. The values in the pink bars are the heating powers generated for each state in the sample heater ON status. **c,** Abridged general view of the experimental setup and procedure. The time profile of $T_{base}$ and power generated by the heater are sketched in the lower panel.

## Supplementary Note 4: Thermodynamic properties under fields perpendicular to the honeycomb plane.

Our thermodynamic measurements under out-of-plane magnetic fields found relatively

smooth $M(B)$ curves in the investigated parameter range. However, the field derivative $dM/dB$ highlights their non-linearity. Similarly to the magnetization, the magnetostriction curves also show non-linearity, which points to competing magnetic and elastic energy scales.

As mentioned in the main text, a recent work of thermodynamic measurements performed up to higher magnetic fields found anomalies attributed to phase transitions [31], which match the features of our $\kappa(B)$ isotherms. These anomalies are out of range of the fields reached in Supplementary Fig. 4.

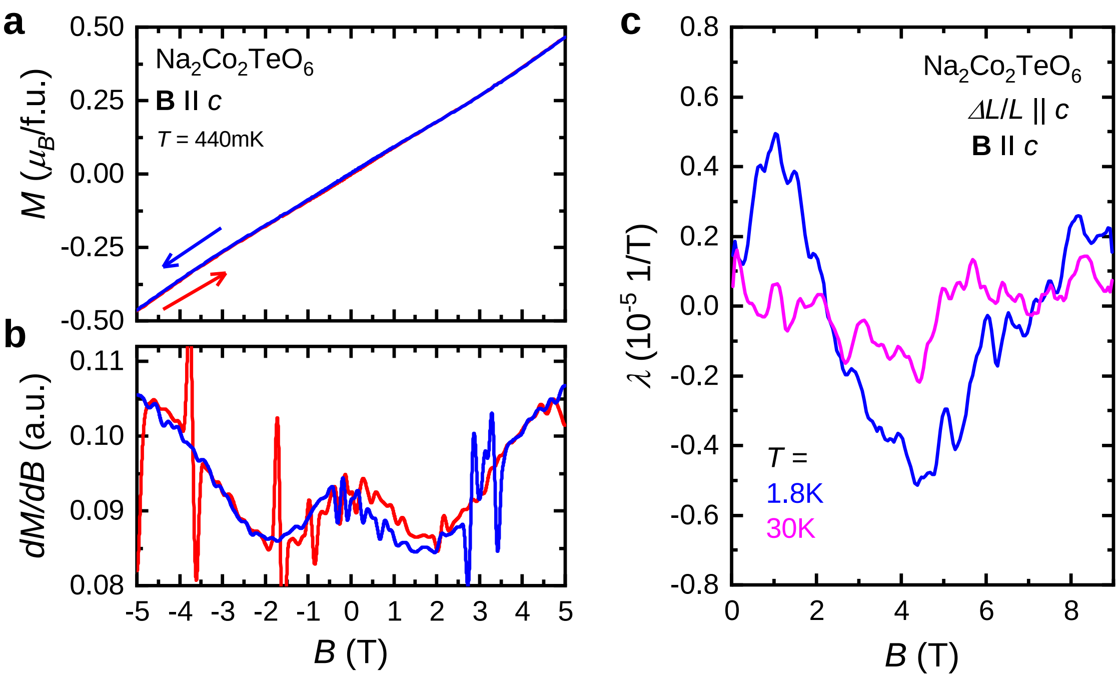


**Supplementary Figure 4 | Thermodynamic properties of NCTO under fields perpendicular to the honeycomb plane. a,** Magnetic field dependence of the magnetization at 440 mK ($\mathbf{B} \parallel c$). The magnetic field was applied in both $+c$ and $-c$ directions up to 5 T. The field derivative $dM/dB$ is shown in panels **b,** and **c.** Longitudinal magnetostriction measured at 1.8 K and 30 K along the $c$ axis ($\Delta L \parallel c$) with magnetic field applied along the $c$ axis ($\mathbf{B} \parallel c$), too.
